# Supplementary material for: zonoLAB: A MATLAB toolbox for set-based control systems analysis using hybrid zonotopes
Source: arXiv:2310.15426 source file (2024-06-10)
Supplement: Supplementary file 1 [file 06_Appendix.tex]

\section*{APPENDIX}
% Appendixes should appear before the acknowledgment.

\subsection*{Plotting}

\subsection*{Functional Decomposition}

\subsection*{Redundancy Removal}

% \section*{ACKNOWLEDGMENT}

% Some Acknowledgments. 
